# Supplementary material for: Dictionary-Free MRI PERK: Parameter Estimation via Regression with Kernels
Source: arXiv:1710.02441 source file (2017-10-06)
Supplement: Supplementary file 1 [file supp.tex]

% reset counters for supplement
\setcounter{section}{0}
\setcounter{equation}{0}
\setcounter{figure}{0}
\setcounter{table}{0}
\setcounter{page}{1}
\makeatletter

% supplement headers
